# Supplementary material for: Spatiotemporal Visualization of Long-Range Anisotropic Plasmon Polaritons in Hyperbolic MoOCl2
Source: arXiv:2506.13719 ancillary file (2026-02-27)
Supplement: Supplementary file 1 [file HyperbolicSurfacePlasmons_MoOCl2_SI_Arxiv.pdf]

# Supplementary Information for “Direct visualization of visible-light hyperbolic plasmon polaritons in real space and time”

Atreyie Ghosh,<sup>1,\*</sup> Calvin Raab,<sup>1,2,\*</sup> Joseph L. Spellberg,<sup>1,2</sup> Aishani Mohan,<sup>1,2</sup> and Sarah B. King<sup>1,2,†</sup>

<sup>1</sup>*James Franck Institute, The University of Chicago, Chicago, IL 60637, USA*

<sup>2</sup>*Department of Chemistry, The University of Chicago, Chicago, IL 60637, USA*

(Dated: June 16, 2025)

## Table of Contents

### I. Supplementary Discussion

- I A. Polarization calibration
- I B. FDTD Simulations
- I C. Fourier Filtering of Time-Resolved Data
- I D. Phase Velocity Measurement
- I E. Group Velocity Measurement
- I F. Calculations of Propagation Lengths
- I G. Polarized Raman Spectroscopy

### II. Supplementary Figures

- S12. Characterization of MoOCl<sub>2</sub> flakes
- S13. Dispersion Calculations
- S14. Static PEEM at 396 and 516 nm
- S15. Schematic of Interferometer for Time-Resolved Experiments
- S16. Power Dependence of PEEM Images

---

\* These two authors contributed equally.

† sbking@uchicago.edu

## I Supplementary Discussion

### A Polarization Calibration

The PEEM sample is illuminated via pulsed laser that is reflected from a near-normal incidence (NNI) rhodium mirror inside the PEEM column. The angle of incidence is  $4^\circ$  from normal, which means the electric field is effectively parallel to the sample plane and rotation of the laser polarization outside the chamber results in the rotation of the electric field in the sample plane. To calibrate the angles of the  $\lambda/2$  plate (HWP) to the polarization in our PEEM images we use a monolayer graphene/300 nm  $\text{SiO}_2/\text{Si}$  substrate. The reflectivity of Rhodium is maximized for s-polarized light and minimized for p-polarized light. Therefore the laser polarization angle at which the total photoelectron count is maximized is taken to be s-polarized with respect to the Rh mirror, and corresponds to the vertical axis of the PEEM image ( $0^\circ$  with respect to vertical).

By fitting the total intensity of the photoemission yield as a function of HWP angle to a function  $f(x) = A \cos^2(k * (x - \phi)) + D$  where  $\phi$  then corresponds to s-polarized light, as shown in Figure S1A, we can create a calibration curve to connect the angle of the laser polarization in our PEEM images with that of the HWP angle outside of the chamber, Figure S1B. Longer discussions regarding this calibration and how to correct for relative intensities in a polarization-dependent experiment can be found in references Joshi *et al.* [1], Spellberg *et al.* [2].

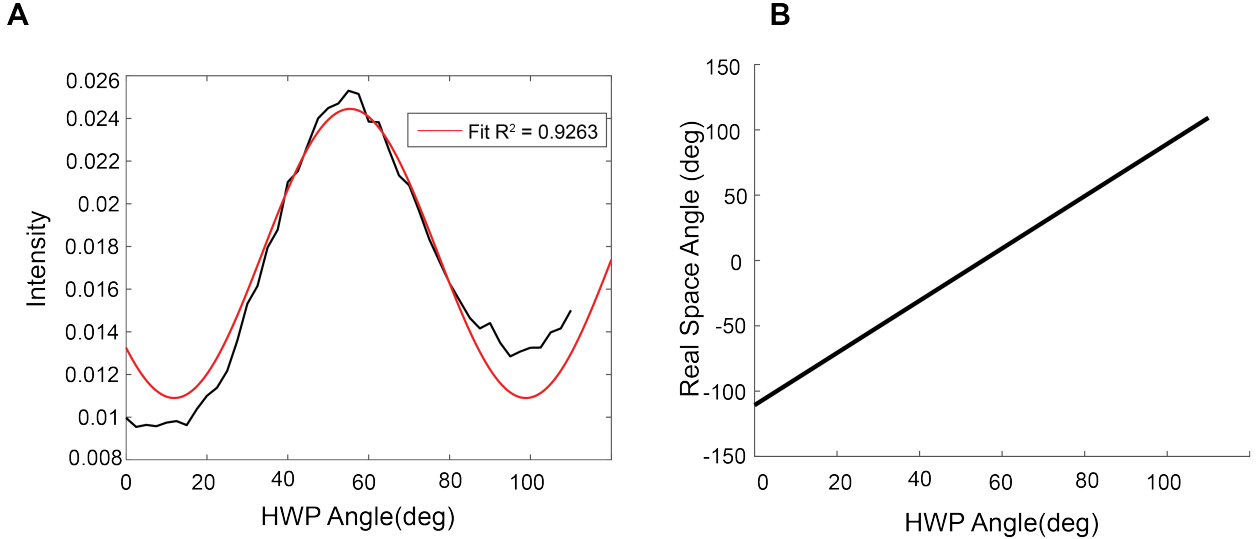

**FIG. S1:** (A) Measured photoemission intensity as a function of HWP angle fit with a  $\cos^2$  function as described in the text. (B) Calibration of the  $\frac{\lambda}{2}$  plate angle to the real space angle.

### B FDTD Simulations

For the Finite Difference Time Domain (FDTD) simulation corresponding to Figure 2F (for  $\text{MoOCl}_2$ ), we introduced three well-spaced half circular curves along the edge of a 200 nm  $\text{MoOCl}_2$  thin film on Si substrate with native oxide and simulated the PEEM response following a previously reported method [3]. In contrast, Figure S2A shows the same simulation but performed on a 200 nm thick Ag film as a reference. Unlike the hyperbolic focusing observed for  $\text{MoOCl}_2$ , Ag displays spherical and diverging wavefronts, consistent with its isotropic optical properties. This distinction is further highlighted in a second set of simulations (Figure S2B), where instead of modifying the thin film edges, we introduced a half circular coupling structure (radius  $1.5 \mu\text{m}$ ) directly on the surfaces of both  $\text{MoOCl}_2$  (left) and Ag (right). While  $\text{MoOCl}_2$  again demonstrates hyperbolic focusing behavior of surface plasmon mode, Ag continues to exhibit spherical wavefronts. These results underscore the material-dependent nature of plasmon propagation and highlight the potential for controlled hyperbolic focusing in  $\text{MoOCl}_2$ , which will be explored in more detail in future work.

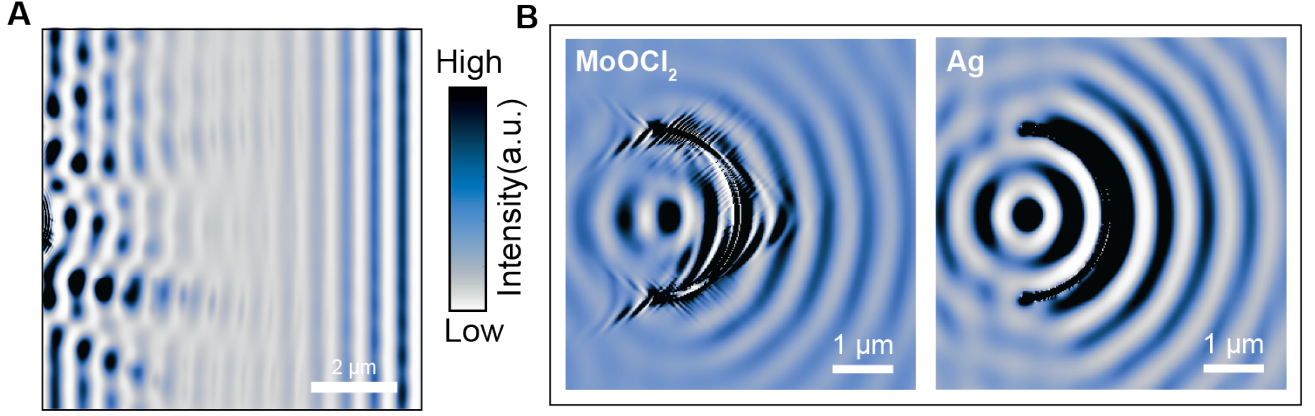

**FIG. S2:** (A) PEEM image reproduced from FDTD simulation for an Ag thin film of thickness 200 nm with curved edges and all identical parameters used for a MoOCl<sub>2</sub> flake shown in Figure 2F. (B) FDTD reproduced PEEM images of a MoOCl<sub>2</sub> (left) and Ag (right) thin films with a half-circular coupling structure of radius 1.5 μm etched on surface under laser illumination of wavelength 774 nm.

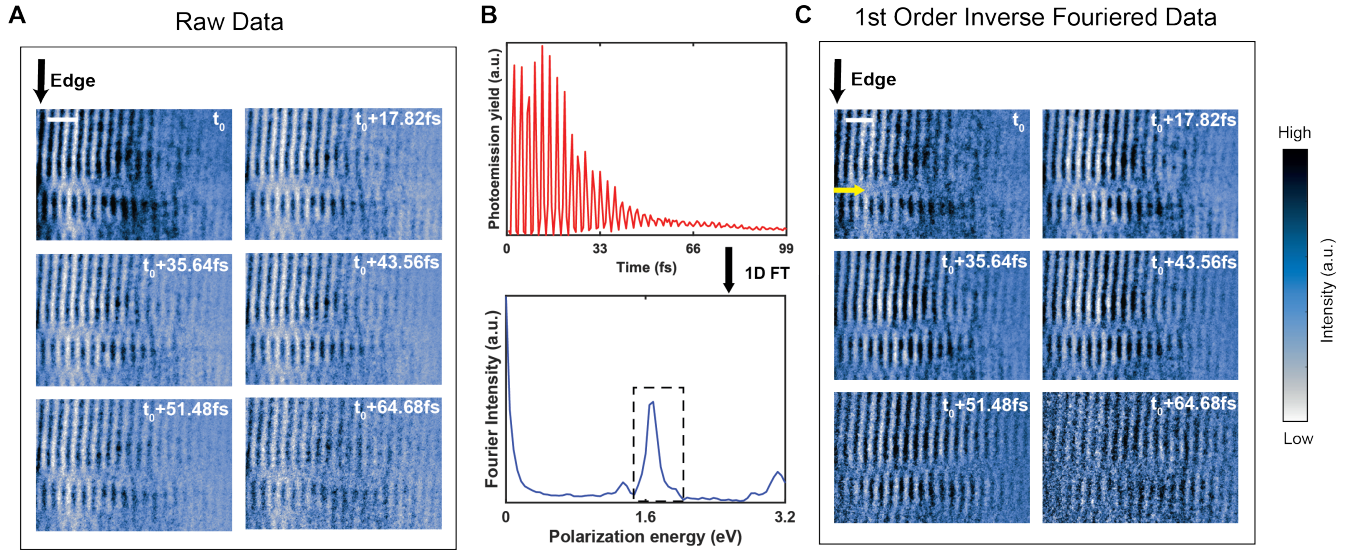

**FIG. S3:** (A) Raw PEEM images from time-resolved experiment shown in Figure 1C, acquired from the same flake discussed in Figure 3.  $t_0$  corresponds to temporal overlap of the pump and probe pulses. The timestamps indicate the pump-probe delay and the color scale represents photoelectron yield. The edge of the flake is on the left side of each image, marked by a black arrow. (B) The top panel shows the time-resolved photoemission signal (red) integrated over the spatial region highlighted in (A). A one-dimensional Fourier transform (FT) is performed along the time axis to convert the data into the energy domain. The lower panel shows the resulting FT amplitude (blue) as a function of the polarization energy,  $\hbar\omega$ . A square window (black dashed box), center at  $1\hbar\omega$ , denotes the energy range for the inverse FT. (C) First-order inverse Fourier transformed images, corresponding to raw data in (A), isolate the first order light-plasmon interaction. These images reveal plasmon propagation from left to right over time, highlighted by the yellow arrow. Scale bars in (A) and (C) indicate 2 μm.

### C Fourier Filtering of Time-Resolved Data

In an interferometric time-resolved PEEM experiment (Figure 1C) with incident laser wavelength 774 nm (1.6 eV), incident pump-probe excitation generated a delay ( $\Delta t$ ) dependent signal that captures the interference between the SPP wavepacket initiated by the pump pulse and the optical field of the delayed probe pulse. As a result, the time-resolved PEEM technique maps the flow of SPPs across the material surface. Figure S3A shows raw time-resolved PEEM images beginning at  $t_0$ , when the pump and probe temporally overlap. These images reflect delay-dependent photoemission yield (top panel of Figure S3B, profile in red) arising from a nonlinear coherent absorption process from multiple photons of energy  $\hbar\omega$ , where  $\omega$  is driving frequency of laser. Due to the interference between pump and probe

induced fields, the signal intensity oscillates, allowing decomposition of each pixel into different harmonic components of the excitation field. The raw data contains both the dynamic interference pattern and a static photoemission background, primarily attributed to the unmodulated out-of-plane component of the SPP field. To isolate the dynamic contribution, a pixel-wise one-dimensional Fourier transform (FT) is applied to the raw data series (bottom panel of Figure S3B, profile in blue) from time to energy domain [4, 5]. A square filter (black dashed box in Figure S3B) is then used to extract the  $1\omega$  component, which is subsequently inverse Fourier transformed to generate the filtered images shown in Figure 3 and Figure S3C. These images are phase-locked to the incident laser field oscillation with a periodicity of 2.6 fs. This approach parallels the techniques used in interferometric multi-photon photoemission spectroscopy [6]. The resulting  $1\omega$  images visualize how the interference between the pump-induced SPP and the probe field evolves with increasing  $\Delta t$ . In other words, Figure S3C captures the time-resolved, first order optical-SPP interaction, specifically the interference between the probe field and the in-plane component of the pump-excited SPP field. As a result, unlike the raw images, the plasmon propagation is prominent in the first order images in Figure S3C. The edge of the flake is located on the left side of each image, denoted by the black arrow. At  $t_0$ , SPPs are launched from the left edge and with increasing  $\Delta t$ , they propagate from left to right, as highlighted by the yellow arrow.

#### D Phase Velocity Determination

The phase velocity was determined by extracting the peak positions from the linecut shown in Figure 3C of the main text and fitting it to a straight line, Figure S4A. The slope of the linear fit is  $0.98 \pm 0.07 c$ , representing the phase velocity. Theoretically the phase velocity is defined as  $v_p = \omega \cdot k_x$ . Figure S5 shows the calculated  $v_p$  as a function of energy from the calculated HPP dispersion based on the published dielectric function in Zhao *et al.* [7]. At 1.6 eV, the theoretical  $v_p$  is  $0.96 c$ , which is in well agreement with the experimental value. As a complementary approach, we also estimated the average periodicity of the surface plasmon modes from the intensity profile across the yellow line of the PEEM image shown in Figure 3B at  $t_1$  but for an extended horizontal dimension. The average peak-to-peak spacing was measured to be 728 nm (Figure S4B). Given the excitation wavelength of 774 nm, the associated angular frequency is  $\omega = 2.435 \times 10^{15}$  rad/s. Using the relation  $v_p = \omega \lambda / 2\pi$ , we obtain  $v_p$  of  $0.94 \pm 0.04 c$  within error bars of our direct calculation for time-resolved data.

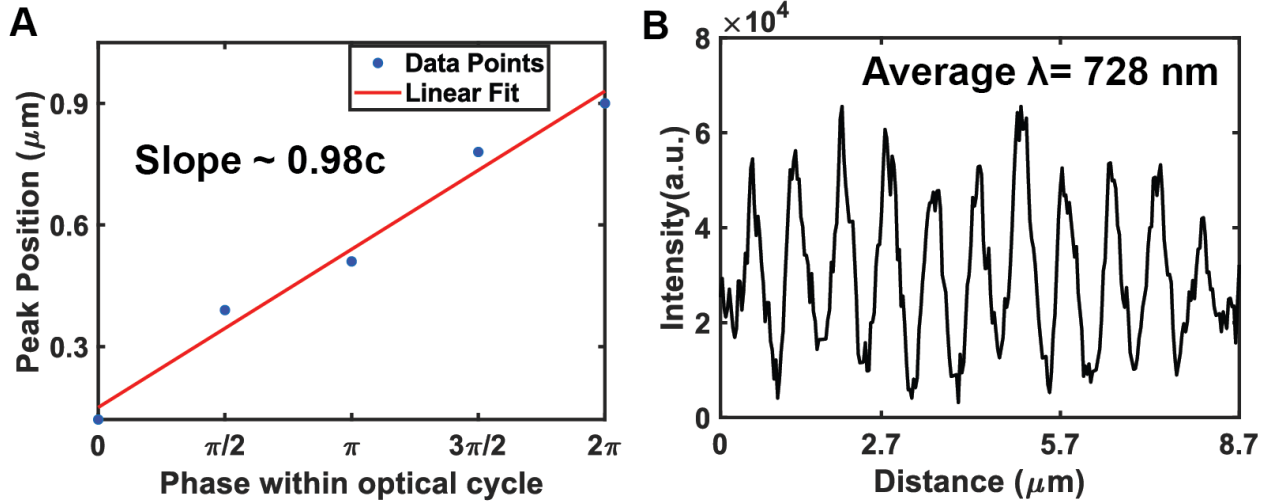

**FIG. S4:** (A) Linear fit of the peak position along the dashed line in Figure 3C as it shifts right with the progression of an optical cycle. The extracted slope is approximately  $0.98c$ , corresponding to the phase velocity ( $v_p$ ) with a standard deviation  $0.07c$ . (B) Intensity profile of the PEEM image in Figure 3B at  $t_1$  across the yellow line but for extended  $x$  dimension. The average peak periodicity is 728 nm. The associated  $\omega$  value is  $2.435 \times 10^{15}$  rad/s for a 774 nm laser (used for the experiment), providing a phase velocity value of  $0.94c$ .

#### E Group Velocity Determination

The group velocity,  $v_g$ , of the traveling plasmon wave-packet can be calculated from the momentum-resolved dispersion relation for HPPs in  $\text{MoOCl}_2$  or from spatiotemporal analysis of the time-resolved PEEM measurements.

Theoretically, the group velocity of an optical mode is given by  $v_g = \frac{\partial \omega(k)}{\partial k} = \frac{1}{\hbar} \frac{\partial E}{\partial k}$ . Using the calculated dielectric function from [7], both the group and phase velocity may be determined from the calculated plasmonic dispersion (Figure S5).

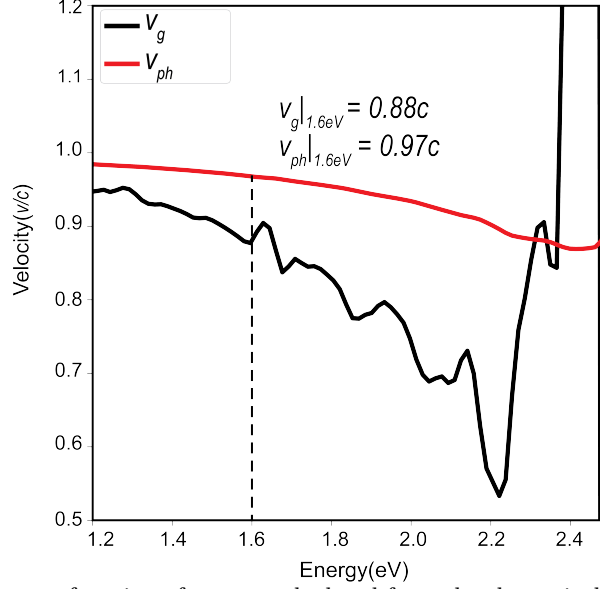

**FIG. S5:** Group and phase velocity as a function of energy calculated from the theoretical dielectric function [7]. The respective group and phase velocities at 1.6 eV are  $0.88c$  and  $0.97c$ .

To determine the group velocity directly from our time-resolved PEEM measurements, a line profile of PEEM intensity was extracted along the  $a$  axis of a  $\text{MoOCl}_2$  flake for each time step in a time resolved PEEM experiment, as shown in Figure 3 of the main text. To account for spatially dependent changes in PEEM intensities within each optical cycle, the linecut was drawn after second order polynomial background subtraction and normalization for each frame. To extract the envelope of the wave-packet, first each profile was converted to a positive intensity with respect to its mean with

$$I_{PE}^+ = |I_{PE} - \text{mean}(I_{PE})|. \quad (\text{S1})$$

Figure S6(A) shows an example of  $I_{PE}^+$  at  $t = 53$  fs. Next, each profile was Fourier transformed and the high frequency ( $> 0.5 \mu\text{m}^{-1}$ ) components were filtered out, Figure S6(B). Finally, inverse Fourier transform was applied to the filtered signal to recover the wave-packet envelope. It was fit to a Gaussian in order to find the peak center, Figure S6(C).

We then applied this procedure to the data at every time step. Spacetime diagrams of the original data, after converting to  $I_{PE}^+$ , and after applying the Fourier filter are shown in Figures S7(A,B,C). There are three distinct segments in the data: at early times the wave-packet appears stationary, at intermediate times there is propagation, and at late times there is no longer a clear wave-packet to track. The intermediate time region is used for calculating  $v_g$ .

The Gaussian fitting is mostly robust across the dataset, but at some time steps the fitting failed. Figure S8(A) shows the  $R^2$  of the fitting at each time step. Only fits with  $R^2 > 0.8$  were used in calculating  $v_g$ . Figure S8(B) shows the measured peak centers overlaid on the spacetime diagram. Blue points are used in the velocity calculation and the red points are those that were removed by the  $R^2$  filter.

To calculate  $v_g$ , the data was truncated to remove values after  $t = 64$  fs. Next, the transition point between the early time, stationary behavior and intermediate time propagation was found using a two segment linear regression [8, 9]. This was found to occur at  $t = 44$  fs. The data was then fit to a line in each region. The early time velocity was found to be  $0.04 \pm 0.07c$  (essentially stationary) while the later time velocity  $0.69 \pm 0.09c$ . These fits are shown in Figure 3E of the main text.

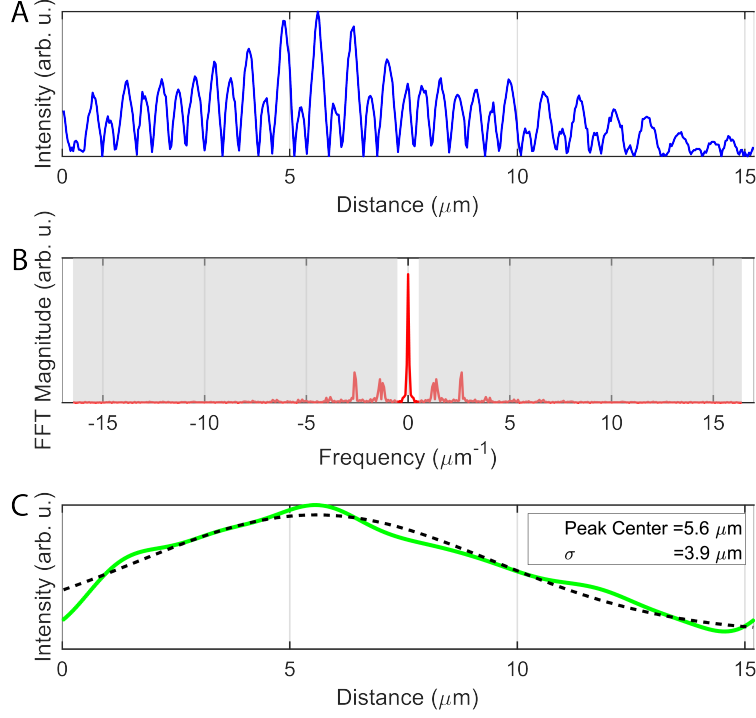

**FIG. S6:** (A) Photoemission emission intensity along the linecut in region marked by the white box in Figure 3(A) of the main text at  $t = 53$  fs after converting to  $I_{PE}^+$ . (B) FFT of the data in (A). Grey shading shows the components that are filtered out ( $> 0.5 \mu\text{m}^{-1}$ ). (C) Inverse FFT of the filtered data (green points) and Gaussian fit (black dashed curve).

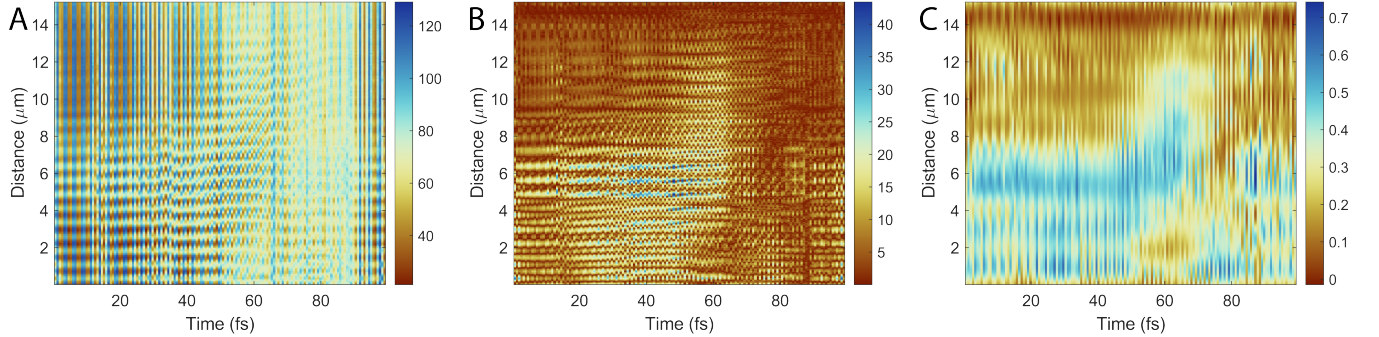

**FIG. S7:** Spacetime diagrams of (A) original data, (B) after converting to  $I_{PE}^+$ , and (C) after applying the Fourier filter. The colorbar indicates intensity (arb. u.).

## F Propagation lengths and Q factors

The plasmonic propagation length is related to the imaginary component of the momentum by  $L_{spp} = \frac{1}{2\Im k_x}$ . It is also related to the plasmonic lifetime ( $\tau$ ) and the group velocity ( $v_g$ ) by  $L_{spp} = \tau v_g$ . A related quantity is the quality factor ( $Q = \frac{\Re k_x}{\Im k_x}$ ) which describes how many optical cycles the plasmon will undergo before decaying.

We determined approximate experimental propagation lengths in three ways, (1) from our static PEEM data, (2) from experimental determinations of the plasmon lifetime and group velocity, and (3) from direct observation of the spatial propagation of a plasmon wave packet. We'll note that because of the limited size of the flakes we were able to make via mechanical exfoliation and viscoelastic stamping, none of these methods provide a definitive upper bound of the propagation length.

1. Using linecuts of static PEEM images we fit the intensity as a function of distance to a decaying exponential. The propagation lengths from this method are shown as a function of energy in Figure S9, between 2-5  $\mu\text{m}$ .

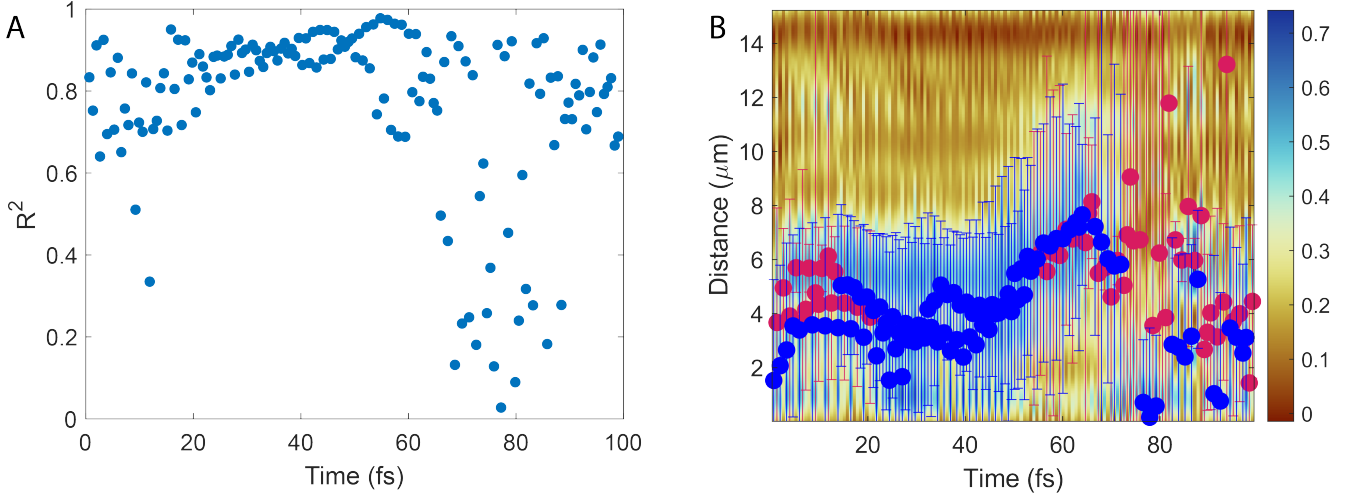

**FIG. S8:** (A) Goodness of fit for the Gaussian envelope found at each time step. Measured peak center position at each time step overlaid on the FFT filtered spacetime diagram. Blue points are for fits with  $R^2 > 0.8$  and red are for  $R^2 < 0.8$ . Error bars are the standard deviation  $\sigma$  from the Gaussian fitting.

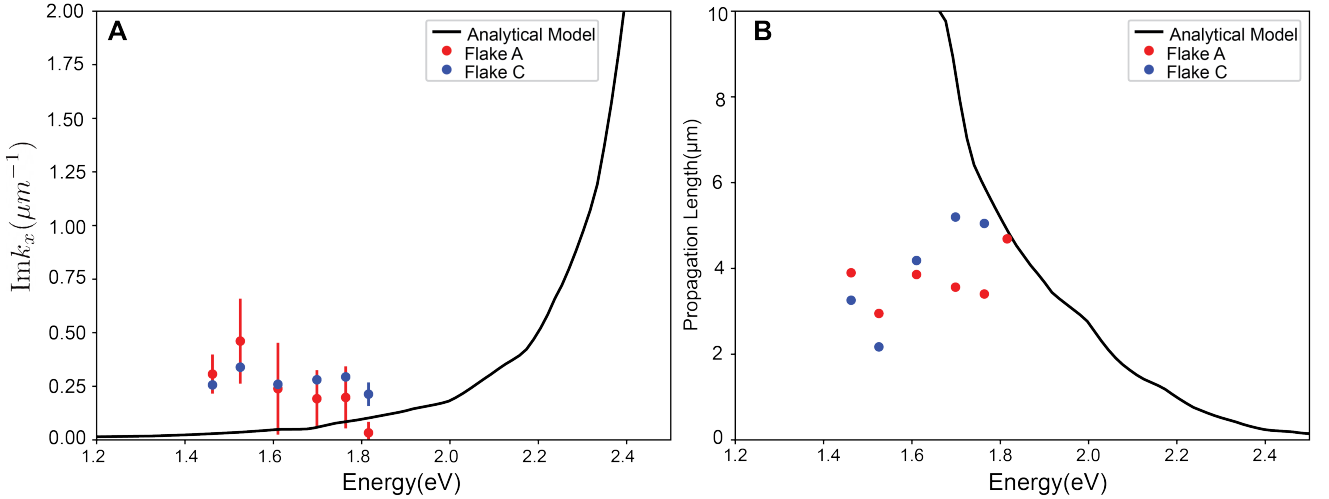

**FIG. S9:**  $\text{Im} k_x$  and propagation length from static PEEM data and analytical models

There is no clear wavelength dependence, suggesting that this is a lower bound on the propagation length due to our short pulse lengths. In other words, the distance over which we see evidence of the plasmon wavepacket is determined more by the length of our laser pulse rather than the true propagation length of the plasmon.

- From our time-resolved data on Flake B, we fit the long time decay to an exponential to recover an estimate of the plasmonic lifetime ( $\tau$ ) of  $33 \pm 5$  fs. The carrier wave has been removed by Fourier transform filtering to make fitting easier. Crucially, we rely on capturing the plasmon-plasmon at long time, rather than the light-light interaction close to  $t_0$  that gives rise to the Gaussian autocorrelation. Combined with the experimentally determined group velocity of  $0.69 \pm 0.09 c$ , this suggests a propagation length of approximately  $7 \mu\text{m}$ .
- In flake B shown in Figure 4, the HPPs propagate for at least twice the flake width ( $30 \mu\text{m}$ ) as they reflect and bounce back, suggesting an even longer propagation length on the order of  $30 \mu\text{m}$ .

More accurate determination of the lifetime and propagation length of HPPs in  $\text{MoOCl}_2$  requires much larger flake sizes and intentionally controlled gratings to launch plasmonic excitations combined with transient grating experiments as shown in [10], out of the scope of the current work.

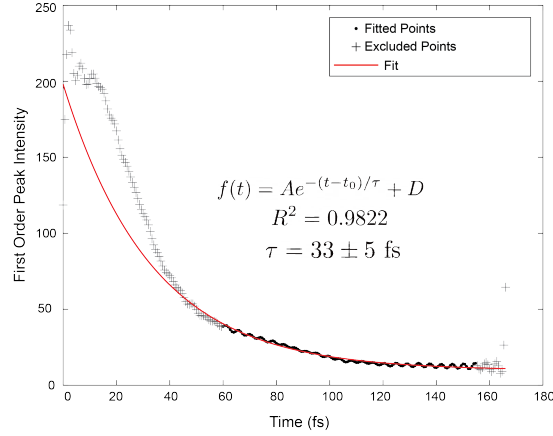

**FIG. S10:** Fitting long time plasmon-plasmon interaction for estimate of plasmonic lifetime ( $\tau$ )

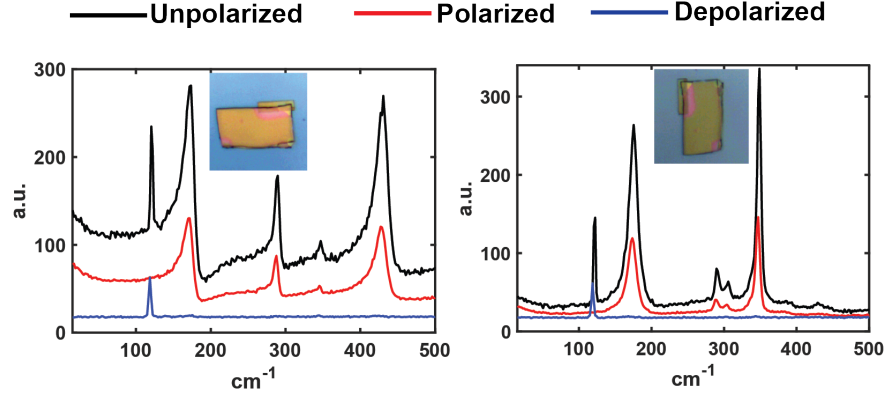

**FIG. S11:** Polarized Raman spectra of  $\text{MoOCl}_2$  flakes at room temperature using 532 nm laser excitation. Spectra recorded without an analyzer are shown in black; those with the polarizer and analyzer in a parallel configuration are shown in red; and depolarized spectra (with polarizer and analyzer perpendicular) are shown in blue. Insets show optical images of the measured flake, with the incident laser polarization oriented vertically. For left panel,  $a$  axis of the flake is aligned perpendicular to the incident laser polarization direction whereas in right panel  $a$  axis is parallel to the laser polarization.

## G Polarized Raman Spectroscopy

To complement polarization-dependent PEEM measurements shown in Figure 2A-B, we performed polarization-resolved Raman spectroscopy on a  $\text{MoOCl}_2$  flake at room temperature with a 532 nm laser with a vertically oriented linear polarization. In the left panel, the Raman spectra correspond to the flake with its  $a$  axis oriented perpendicular to the laser polarization, while the right panel shows the spectra with  $a$  axis parallel to the polarization direction. Two key observations emerge from these measurements. First, the unpolarized Raman spectra (black) exhibit distinctively different vibrational modes depending on the flake's crystallographic axes to the laser polarization, reflecting the strong in-plane anisotropy in  $\text{MoOCl}_2$ . Second, for each flake orientation, the unpolarized Raman spectrum can be viewed as the sum of the polarized (red) and depolarized (blue) spectra, indicating that prominent Raman-active modes are present along both  $a$  and  $b$  axes of the crystal. These initial polarization dependent Raman measurements establish the basis for a more comprehensive investigation of highly anisotropic vibrational properties of  $\text{MoOCl}_2$ . A detailed mode assignment and full spectral analysis will be pursued in future work.

## II Supplementary Figures

### A Characterization of $\text{MoOCl}_2$ flakes

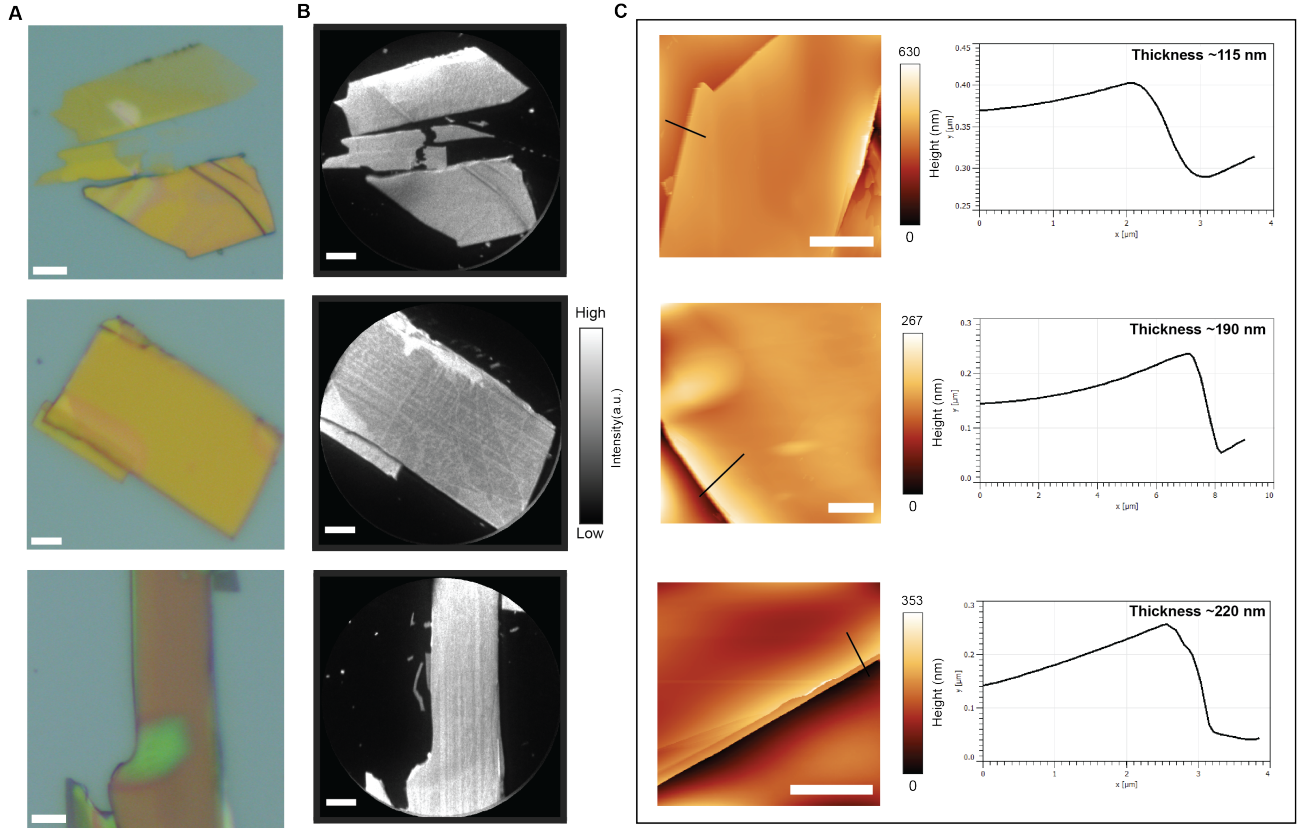

**FIG. S12:** (A) Optical microscope images of three exfoliated 2D  $\text{MoOCl}_2$  flakes on Si substrate presented in this study. (B) Hg lamp PEEM images of the same flakes as in (A) obtained through one photon photoemission process. (C) Atomic Force Microscopy (AFM) images (left panel) of the same flakes along with corresponding height profiles across the black solid lines. Based on the AFM measurements, the thicknesses of the flakes (top to bottom panels) are  $\approx 115\ \text{nm}$ ,  $190\ \text{nm}$  and  $220\ \text{nm}$ , respectively. All the scale bars indicate  $5\ \mu\text{m}$ .

## B Dispersion Calculations

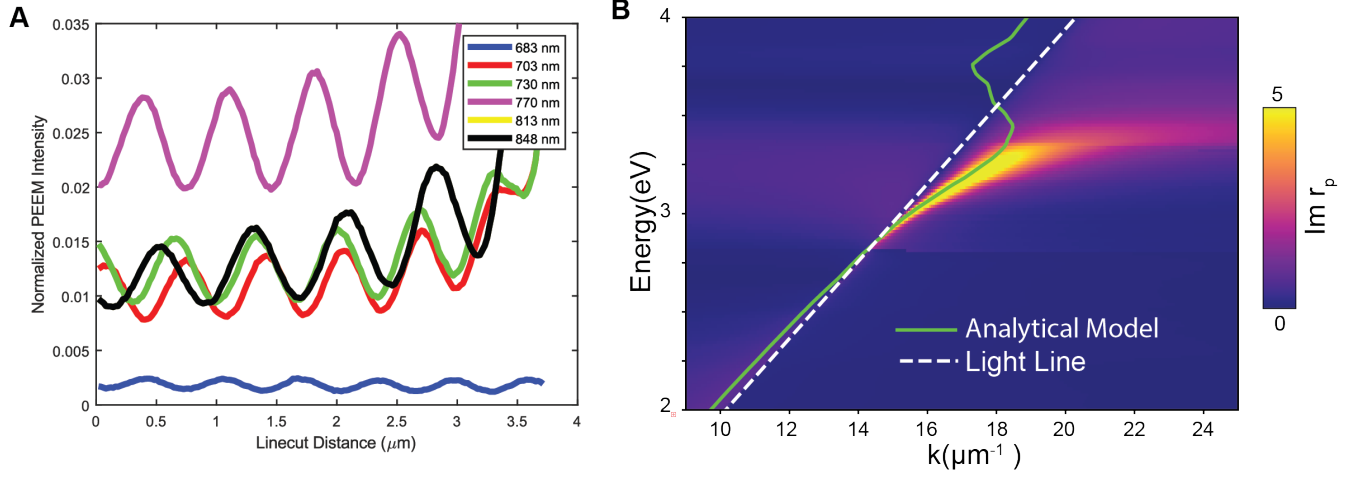

**FIG. S13:** (A) Experimental line cuts from flake A as shown in Figure 2A-C in the main text. (B) Calculated dispersion from the dielectric function in Zhao *et al.* [7] along the  $b$  crystal axis where we observe no plasmonic fringes for comparison to the dispersion along the  $a$  axis shown in Figure 2 of the main text.

### C Static PEEM at 396 and 516 nm

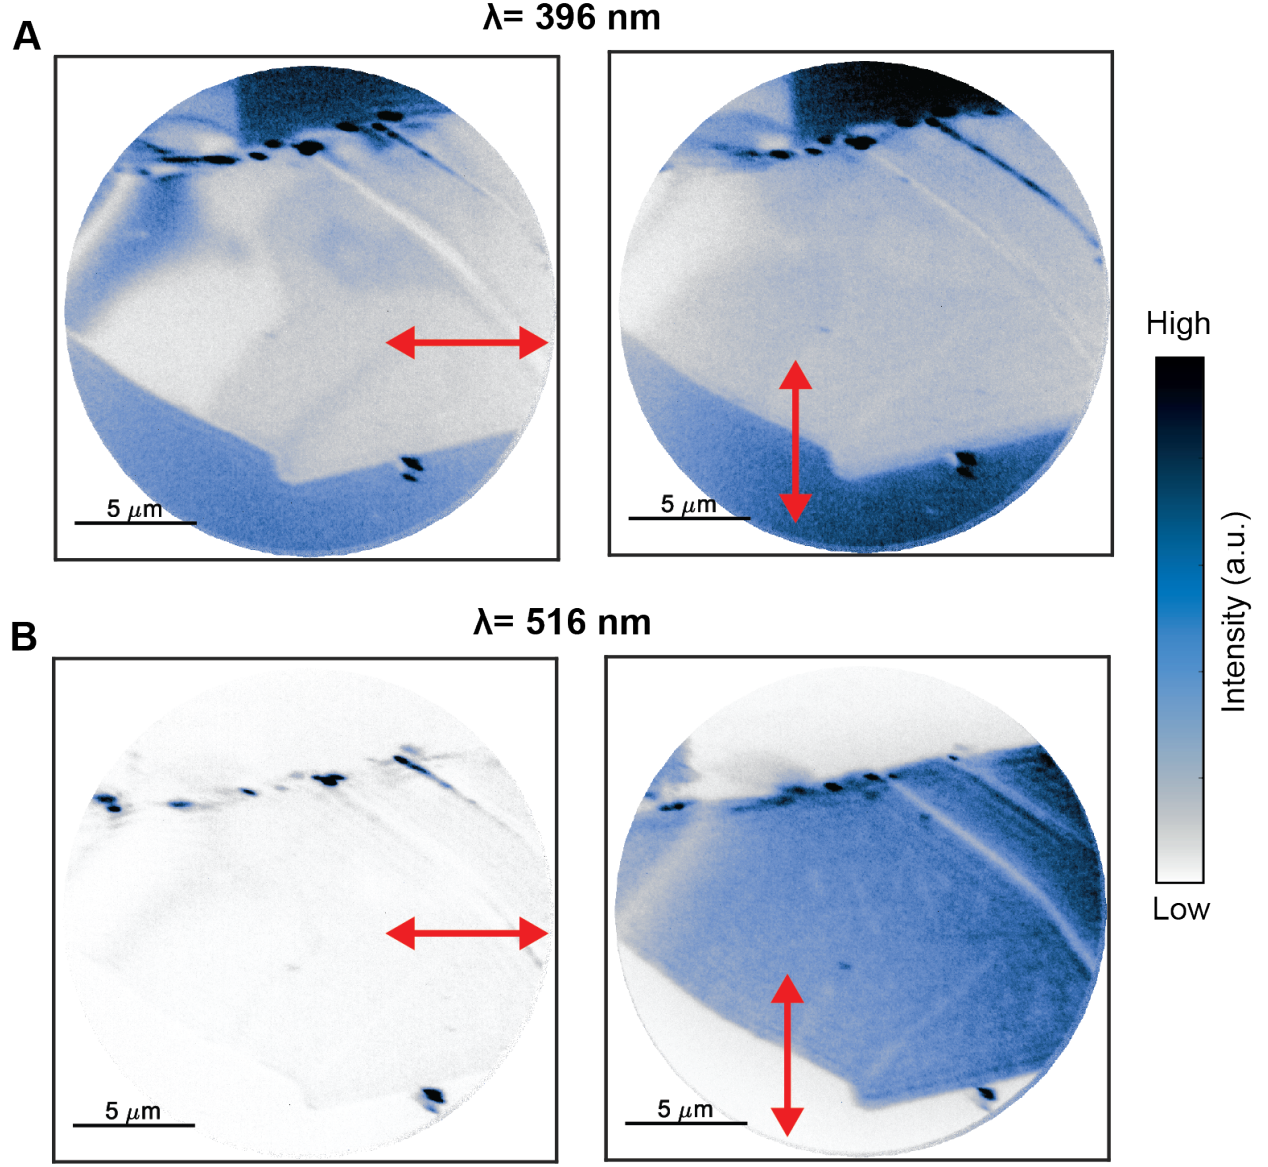

**FIG. S14:** Static PEEM images of the same  $\text{MoOCl}_2$  flake shown in Figure 2A-C, captured under laser illumination at (A) 396 nm and (B) 516 nm. Red arrows indicate the incident in-plane laser polarization direction. Unlike visible and near-IR wavelength, in the UV region the in-plane optical anisotropy is not prominent since the PEEM contrast in (A) is identical for both polarizations. Notably, no surface plasmon modes were observed at 396 nm, despite predictions based on the dielectric function of  $\text{MoOCl}_2$  calculated by Zhao et al.[7], likely due to high optical losses in this wavelength. At 516 nm, the polarization dependent contrast is still evident, as seen in Figure 2A and 2B for a near-IR wavelength, although the surface fringes are much weaker and launch from multiple edges of the flake. The surface modulation at this energy likely arises from a different surface mode than HPPs.

# D Schematic of Interferometer

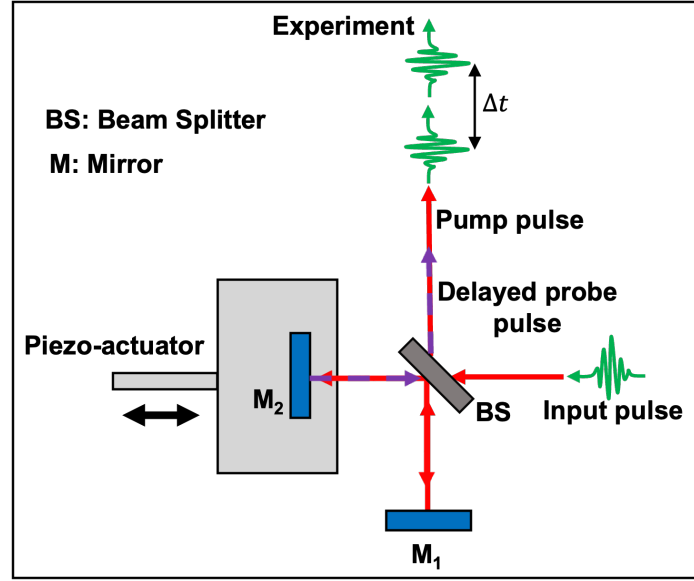

**FIG. S15:** Schematic of the Michelson interferometer used in our experiments for control of the pump-probe delay pulses in the interferometric experiments.

## E Power dependence of PEEM images

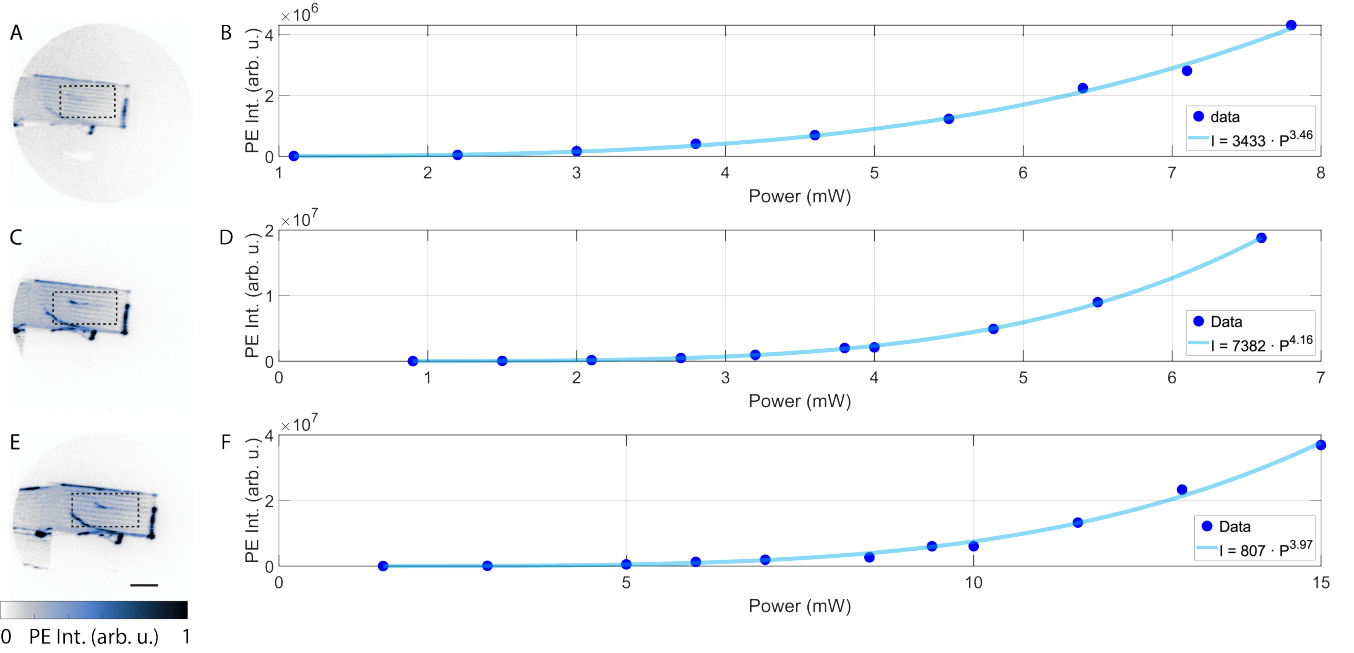

**FIG. S16:** Power dependent PEEM experiments with laser excitation (A,B)  $\lambda = 697 \pm 7$  nm, (C,D)  $\lambda = 773 \pm 10$  nm, and (E,F)  $\lambda = 799 \pm 10$  nm. Points are integrated photoemission intensity from the indicated regions of interest. Curves are fits to  $I = aP^b$ , where  $P$  is the incident laser power and  $b$  is the number of photons in the photoemission process. Scalebar is 5  $\mu\text{m}$ . Power dependent measurements were collected in the same PEEM chamber but with an alternate excitation source (Light conversion Carbide and Orpheus OPA, repetition rate: 100kHz).

- [1] P. P. Joshi, R. Li, J. L. Spellberg, L. Liang, and S. B. King, Nanoimaging of the edge-dependent optical polarization anisotropy of black phosphorus, *Nano Lett.* **22**, 3180 (2022).
- [2] J. L. Spellberg, L. Kodaimati, P. P. Joshi, N. Mirzajani, L. Liang, and S. B. King, Electronic structure orientation as a map of in-plane antiferroelectricity in  $\beta^{\text{I}}$ - $\text{In}_2\text{Se}_3$ , *Sci. Adv.* **10**, eado2136 (2024).
- [3] A. Ghosh, S. Yang, Y. Dai, Z. Zhou, T. Wang, C.-B. Huang, and H. Petek, A topological lattice of plasmonic merons, *App. Phys. Rev.* **8**, 10.1063/5.0062133 (2021).
- [4] Y. Dai, Z. Zhou, A. Ghosh, R. S. K. Mong, A. Kubo, C.-B. Huang, and H. Petek, Plasmonic topological quasiparticle on the nanometre and femtosecond scales, *Nature* **588**, 616 (2020).
- [5] G. Spektor, D. Kilbane, A. K. Mahro, M. Hartelt, E. Prinz, M. Aeschlimann, and M. Orenstein, Mixing the light spin with plasmon orbit by nonlinear light-matter interaction in gold, *Phys. Rev. X* **9**, 021031 (2019).
- [6] M. Reutzel, A. Li, and H. Petek, Coherent two-dimensional multiphoton photoelectron spectroscopy of metal surfaces, *Phys. Rev. X* **9**, 011044 (2019).
- [7] J. Zhao, W. Wu, J. Zhu, Y. Lu, B. Xiang, and S. A. Yang, Highly anisotropic two-dimensional metal in monolayer  $\text{MoOCl}_2$ , *Phys. Rev. B* **102**, 245419 (2020).
- [8] S. Okazaki, Piecewise linear model - file exchange - MATLAB central.
- [9] R. S. Bogartz, A least squares method for fitting intercepting line segments to a set of data points, *Psychological Bulletin* **70**, 749 (1968).
- [10] Y. Gong, A. G. Joly, D. Hu, P. Z. El-Khoury, and W. P. Hess, Ultrafast imaging of surface plasmons propagating on a gold surface, *Nano Lett.* **15**, 3472 (2015).
